# Supplementary material for: NISPA: Neuro-Inspired Stability-Plasticity Adaptation for Continual Learning in Sparse Networks
Source: arXiv:2206.09117 source file (2022-06-18)
Supplement: Supplementary file 1 [file 0_algorithm.tex]

\section{NISPA Pseudocode}
\begin{center}
\begin{minipage}{0.7\linewidth}
 \begin{algorithm}[H]
 \centering
       \caption{NISPA on task $t$ (repeated for every task). $S$ and $S_c$ denote the set of all stable and candidate stable units, respectively.}
       \label{alg:method}
    \begin{algorithmic}[1]
      \REQUIRE $S$, $e$, $a_{f}$, $k$, $M$ \COMMENT{$M$ is the model}
      \STATE $a_{max} \gets 0$, $\tau \gets 1$, $p \gets 1$  \COMMENT{$p$ is the phase index}
       \LOOP
         \STATE $M \gets \textbf{Train}(M, e, D_t)$ \COMMENT{use training set $D_t$}
         \STATE $\text{CacheM}[p] \gets M$ \COMMENT{Store the model}
         \STATE $a \gets \textbf{Validate}(M, V_t)$ \COMMENT{use validation set $V_t$}
         \STATE $a_{max} \gets \max(a_{max}, a)$
         \IF {$a_{max} - a_{f} \leq a $}
             \STATE $\tau \gets \frac{1}{2} \left ( 1 + \cos \left ( \frac{p \times \pi}{k} \right ) \right ) $
             \STATE $S_c \gets \textbf{SelectCandidates}(M, S, \tau)$
             \STATE $\text{CacheS}[p] \gets S \cup S_c$ \COMMENT{Store the set of stable units}
             \STATE{\# Drop connections from $P^l$ to $S^{l+1} \cup S_c^{l+1}$}
             \STATE $M \gets \textbf{Drop}(M, S, S_c)$ 
             \STATE{\# Randomly grow connections from $U^l$ to $P^{l+1}$}
             \STATE $M \gets \textbf{Grow}(M, S, S_c)$ 
             \STATE $p \gets p + 1$ \COMMENT{Increase the phase index}
         \ELSE
            \STATE $M \gets \text{CacheM}[p - 1]$ \COMMENT{Restore saved $M$}
            \STATE $S \gets \text{CacheS}[p - 2]$ \COMMENT{Restore saved stable units}
            \STATE{\# Freeze input connections to units in $S$}
            \STATE $M \gets \textbf{Freeze}(M, S)$ 
            \STATE{\# Reinitialize connections from $U^l$ to $P^{l+1}$}
            \STATE $M \gets \textbf{Reinit}(M, S)$ 
            \STATE \textbf{return} $M$, $S$ \COMMENT{Start task $t+1$}
         \ENDIF
      \ENDLOOP
    \end{algorithmic}
\end{algorithm}
\end{minipage}
\end{center}
