# Supplementary material for: NISPA: Neuro-Inspired Stability-Plasticity Adaptation for Continual Learning in Sparse Networks
Source: arXiv:2206.09117 source file (2022-06-18)
Supplement: Supplementary file 3 [file 2_experiment_details.tex]

\section{Experimental Details}
This section reports experimentation details and hyperparameters for our experiments. 

\subsection{Datasets} 
For all datasets (CIFAR10, CIFAR100, MNIST, EMNIST, and FashionMNIST), we reported the accuracy on the official test sets and used 10\% of the training dataset for validation. We performed early stopping (including early stopping at phase level) based on the validation accuracy. Likewise, we fine-tuned the hyperparameters for NISPA and all baselines using the validation datasets. Furthermore, we have not performed any data augmentation.

\subsection{Hyperparameters} 
We trained all models using Adam optimizer unless otherwise indicated. Furthermore, we used early stopping on the validation dataset to determine the number of epochs. We fairly searched the hyperparameters for all baselines and reported each method's best performance. Our hyperparameter search space included officially used hyperparameters in the dataset if available.

NISPA comes with the following hyperparameters:
\begin{itemize}
    \item $e$ is the number of epochs for each phase.
    \item $a_f$ is the validation accuracy loss we are willing to accept.
    \item $k$ is a hyperparameter for the cosine annealing function that governs step size for $\tau$.
    \item $d$ is the density level for our model. Note that if this is relatively high (e.g., 80\%), our method does not guarantee a constant density level since growing for every dropped connection becomes impossible. In other words, NISPA tends to prune the network if the initial network is dense.
\end{itemize}

NISPA is not sensitive to any of these hyperparameters. They only determine inevitable trade-offs. For example, decreasing $a_f$ puts more emphasis on early tasks and results in more aggressive freezing, reducing the number of available units for future tasks. On the other hand, $e$ and $k$ determine the number of epochs. For instance, smaller $k$ decreases $\tau$ faster, resulting in few phases, decreasing the number of epochs in which the model is trained. \textbf{Figure}~\ref{fig:cos_anl} shows the shape of the  cosine annealing function for various $k$ values. Finally, we observed that density between 0.05 and  0.2  tend to be best for NISPA. Extremely low density such as 0.01  hinders the training since the network underfits the given task. On the other hand, denser networks tend to make units highly entangled, making isolation challenging.  \textbf{Table}~\ref{tab:table_hyper} presents all hyperparameters used in the experiments.

\begin{figure}[ht]
\begin{center}
\centerline{\includegraphics[width=8cm]{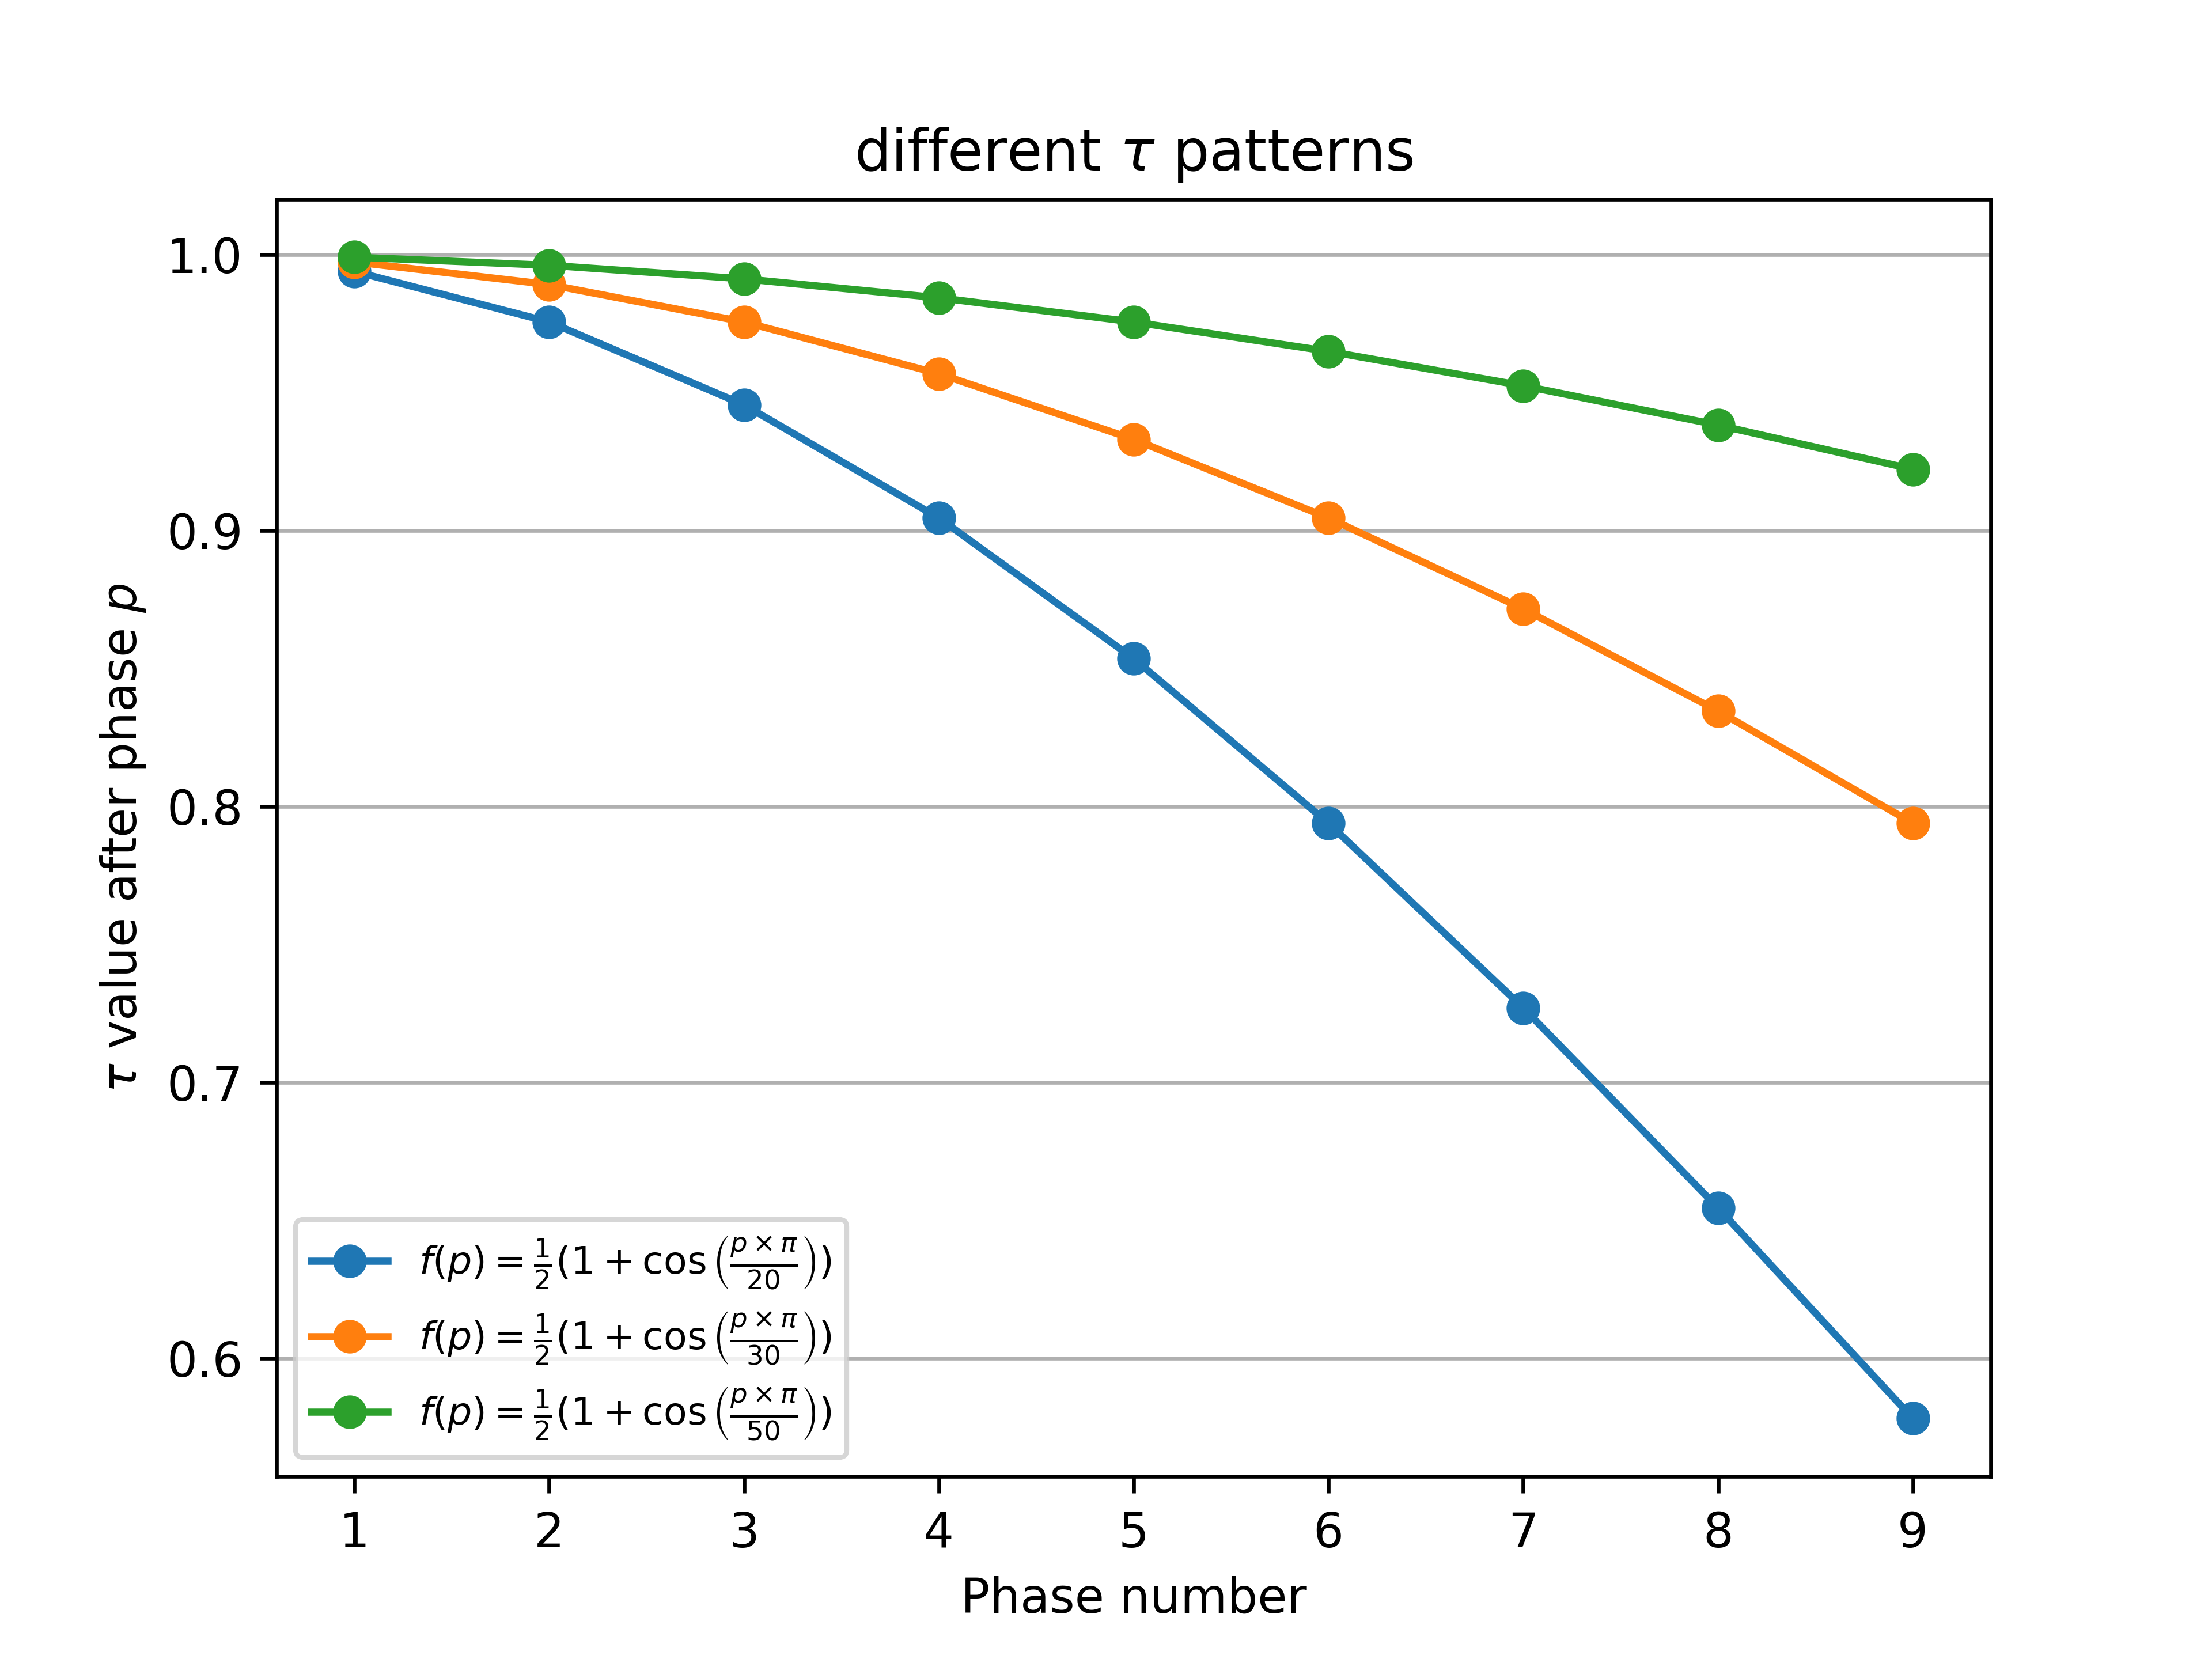}}
\caption{Cosine annealing function.}
\label{fig:cos_anl}
\end{center}
\vskip -0.2in
\end{figure}

\begin{table}[t]
\caption{Hyperparameters for NISPA for each task sequence. Here $\lambda $ is an extra hyperparameter for replay. See section \ref{cil_details} for details.}
\label{tab:table_hyper}
\begin{center}
\begin{small}
\begin{sc}
\begin{tabular}{lcccccccr}
\toprule
Dataset & Learning Rate & Batch Size &  $e$ & $a_f$ & $k$ &  $d$  & $\lambda$ & \\
\midrule
EMNIST + FashionMNIST   & 0.01 & 512 & 5 &  0.75 & 30 &  0.2 &  -- &\\
CIFAR100  & 0.002& 64 & 5 &  2.5 & 30& 0.1& -- & \\
CIFAR10  & 0.002& 128 & 5 &  0.75& 30& 0.1& -- &  \\
Permuted MNIST (5 tasks, 10\%)  & 0.01& 1024 & 2 &  0.75& 40& 0.1 & -- & \\
Permuted MNIST (5 tasks, 100\%)  & 0.01& 1024 & 3 &  0.75& 40& 0.1 & -- & \\
Permuted MNIST (2 tasks)  & 0.01& 256 & 5 &  0.5& 40& 0.25 & -- & \\

Replay MNIST (10 per class)  & 0.05& 512 & 3 &  0.5& 30 & 0.1 & 5 & \\
Replay EF-MNIST (10 per class) & 0.05& 128 & 5 &  1.5& 30& 0.3 & 0.5 & \\
Replay CIFAR10 (10 per class)  & 0.001& 256 & 5 &  2 & 40 & 0.1 & 1 & \\

Replay MNIST (50 per class)  & 0.05& 64 & 3 &  1& 30& 0.1 & 5 & \\
Replay EF-MNIST (50 per class) & 0.1& 256 & 5 &  2.5& 30& 0.3 & 0.5 & \\
Replay CIFAR10 (50 per class)  & 0.001 & 256 & 5 &  1& 40& 0.1 & 7.5 & \\

Replay MNIST (100 per class)  & 0.1& 256 & 5 &  0.5& 30& 0.1 & 5 & \\
Replay EF-MNIST (100 per class) & 0.05& 128 & 5 &  2& 30& 0.3 & 1 & \\
Replay CIFAR10 (100 per class)  & 0.002& 512 & 5 &  2& 40& 0.1 & 5 & \\
\bottomrule
\end{tabular}
\end{sc}
\end{small}
\end{center}
\vskip -0.2in
\end{table}


\subsection{Weight Initialization and Sparsification} \label{initialization}
Weights are initialized using Kaiming's method. Specifically,  they are sampled from a zero-centered Gaussian distribution with a variance inversely proportional to each layer's width: $\sigma_l^2 = \frac{2}{N_l}$. On the other hand, newly grown connections are initialized to small values based on existing connection weights. Formally, for each layer $l$, we compute the mean $\mu_l$  and the standard deviation $\sigma_l$ of the existing weights. Then, at layer $l$, we sample newly added connections weight as $\theta \sim \mathcal{N}_l(\mu_l, \sigma_l)$. 

In all experiments, networks are initially sparsified using unstructured random pruning. So, each connection has an equal chance of removal, and sparsity is uniform across all layers. The only exception is that we have not pruned the first layer in the convolutional architectures. The reason is that given three-channel image input, units in the first layer are connected to input via three connections. As a result, if we prune the network, we will likely create "dead" units at the initial layer. For example, at 0.1 density, units at the first layer will be dead with a probability of 0.729 ($(1 - 0.1)^3 = 0.729$). Therefore, keeping the first layer dense avoids this problem. Note that this change has almost no effect on the total number of connections.


\subsection{Permuted MNIST Experiments} \label{permuted_mnist}
For permuted MNIST task sequences used in sections \ref{reuse} and \ref{alternative}, we always used the standard MNIST as the first task. The following tasks are the same dataset with permuted input features (i.e., MNIST pixels). For each permutation, we randomly selected  $p_r$ of the pixels and shuffled them. In Section \ref{reuse}, we used an MLP with three hidden layers that consist of 400 units each. On the other hand, in section \ref{alternative},  we consider an MLP with two hidden layers, each with 2000 units. 

This architectural change was necessary to ensure that (1) all models reach a similar accuracy on all tasks and (2) always have enough plastic units to stabilize if needed. Otherwise, it is not possible to have a valid comparison. For example, if a model picks fewer stable units but cannot perform like its counterparts, we cannot make a concrete conclusion. 

\subsection{Other Connection Growth Mechanisms} \label{alternative_details}
In section \ref{alternative}, we experiment with two different connection growing mechanisms, namely, {\em Transfer} and {\em Novel}. The {\em Novel} mechanism randomly samples (uniformly) which connection to grow from only type 1 connections. On the other hand, the {\em Transfer} mechanism randomly (uniformly) picks only type 2 connections. However, in corner cases, such as when the number of stable and plastic units is highly imbalanced, there may not be enough available connections belonging to one of the types to grow in order to preserve the degree of density.

To have a fair comparison between different mechanisms, we need to ensure that all models have the same number of parameters (i.e., the same density level). Therefore, we let each growth mechanism select the other type of connections if they have already grown all of their primary connections and still have an additional quota for growing to preserve the density level. For instance, if the Transfer mechanism has grown all type 2 connections but needs additional 100 connections to preserve the same density, it randomly selects 100 type 1 connections. 
