# Supplementary material for: NISPA: Neuro-Inspired Stability-Plasticity Adaptation for Continual Learning in Sparse Networks
Source: arXiv:2206.09117 source file (2022-06-18)
Supplement: Supplementary file 4 [file 3_parameter_comparison.tex]

\section{Stability of NISPA and Comparison of Learnable Parameters}
\textbf{Table}~\ref{tab:std_params} presents the standard deviations of the average task accuracies for 5 runs. CLNP's exact number of parameters slightly varies during training since it drops some connection between tasks. For simplicity, we calculated all multipliers based on the initial number of parameters. We note that the final number of parameters of CLNP is still multiple times larger than NISPA. For example, in our experiments, CLNP has a density of 0.73 before starting task-5 on E+F MNIST, while NISPA has a density of 0.2 throughout the training.

Note that since we are not pruning biases and the first convolutional layer for NISPA (see Appendix \ref{initialization}), the actual difference is not exactly $5 \times$ and $10 \times$.

\begin{table}[h!]
\vskip -0.2in
\caption{Standard deviations of the average task accuracies for 5 runs. Multipliers indicate the number of parameters compared to NISPA.}
\label{tab:std_params}
\begin{center}
\begin{small}
\begin{sc}
\begin{tabular}{lcccr}
\toprule
Methods & E+F MNIST & CIFAR10 & CIFAR100 \\
\midrule
NISPA & 0.15  & 0.19  & 1.30 \\
STL  & 0.10  & 0.06  & 0.30  \\
STL ISO  & 0.11  & 0.43  & 3.81 \\
CLNP  & 0.18 ($4.94 \times$) & 0.67 ($9.94 \times$) & 5.14 ($9.97 \times$)\\
EWC & 2.11 ($4.94 \times$) & 2.43 ($9.94 \times$) & 2.00 ($9.97 \times$)\\
SI  & 0.55($4.94 \times$) & 2.36 ($9.94 \times$) & 1.83 ($9.97 \times$) \\
MAS   & 2.02 ($4.94 \times$) & 1.26 (($9.94 \times$) & 1.97 ($9.97 \times$)\\
\bottomrule
\end{tabular}
\end{sc}
\end{small}
\end{center}
\vskip -0.2in
\end{table}
