# Supplementary material for: NISPA: Neuro-Inspired Stability-Plasticity Adaptation for Continual Learning in Sparse Networks
Source: arXiv:2206.09117 source file (2022-06-18)
Supplement: Supplementary file 5 [file 4_cil_details.tex]

\section{Class Incremental Learning Experiments} \label{cil_details}
We present results for a simple extension that relies on storing a small number of "raw" samples. We evaluate this extended version of NISPA against four baselines using cumulative average accuracy as the metric. Specifically, let $a_j^{end}$ be the model accuracy evaluated on the held-out test set of the j-th task after learning all tasks. Suppose we have $n$ tasks, we report average cumulative accuracy computed as $A = \frac{1}{n} \sum_{i = 1}^{n} a_i^{end}$.

\subsection{NISPA-Replay}

\textbf{Training: } NISPA-Replay splits the loss terms for memory and task samples. Specifically, the new loss function of task $t$ is defined as:
\begin{equation*}
    \mathbb{E}_{(x, y) \sim D_t} \left [ \mathcal{L}_{CE}(y, f(x) \right ] +  \lambda \; \mathbb{E}_{(x, y) \sim M} \left [ \mathcal{L}_{CE}(y, f(x)) \right ]
\end{equation*}
Here, $f$ is the overall network, $D_t$ is the dataset of task $t$, and  $M$ is the memory buffer. Furthermore,  $\mathcal{L}_{CE}$ is the standard cross-entropy loss and $\lambda$ is a trade-off hyperparameter. In other words, for every gradient update, we get samples from the task dataset along with samples from memory and perform one training step.

We observed that the weight initialization at the task boundaries significantly hurts the performance in class incremental learning. This is because assigning random weights to existing units, arbitrarily changes the activation of output units dedicated for future tasks. This random change in activations of some of the output units causes crosstalk in the softmax layer and prevents trained output units (for classes seen so far) from making valid predictions. Therefore, we omitted the reinitialization step for NISPA-Replay.

\textbf{Sampling: } We initialize a fixed-sized buffer, and it is filled with random samples. We only ensure that each class seen so far have an equal number of samples stored. We could implement a more complex strategy for NISPA. However, we aim to show that NISPA itself alleviates forgetting, and its success in class incremental learning is not due to additional tricks we employed in replay or memory. 

\subsection{Datasets and Architectures}
\textbf{Datasets: } EF-MNIST and  CIFAR10 task sequences are as presented in Section \ref{results}. Our MNIST experiment is a standard split MNIST with five tasks where two consecutive digits constitute one task.

\textbf{Architectures: } For EF-MNIST and MNIST, we used an MLP, and for CIFAR10, we used CNN. Both MLP and CNN details are the same as described in Section \ref{results}. Furthermore, NISPA and baselines were initially sparsified using uniform random pruning (each 2D filter is set to zero-matrix, or edge weight is set to zero with equal probability). We use MLP with 0.1 density on MNIST,   MLP with 0.3 density on EF-MNIST, and CNN with 0.1 density on CIFAR10. NISPA hyperparameters are given in \textbf{Table}~\ref{tab:table_hyper}.

\textbf{Optimizer: } For all networks, we tried both Adam and SGD optimizers. We observed that rehearsal baselines (ER, DER, iCaRL, A-GEM) perform better with SGD on all datasets. So, they are trained using SGD. On the other hand, NISPA performs better with SGD on MNIST and EF-MNIST, while on CIFAR10, Adam leads to better performance. Therefore, we chose the optimizer for NISPA based on the dataset.

\begingroup
\begin{table*}[t!]
	\centering
	{\renewcommand{\arraystretch}{1} 
		\resizebox{\textwidth}{!}{%
			\begin{tabular}{lllllllllllll}
				\hline\noalign{\smallskip}\hline\noalign{\smallskip}
				
				Buffer Size & \multicolumn{3}{c}{10 Samples Per Class} &  \vline &\multicolumn{3}{c}{50 Samples Per Class} &  \vline& \multicolumn{3}{c}{100 Samples Per Class} &  \\ 
				\cline{0-12}
				&  MNIST   & EF-MNIST    & CIFAR10   &\vline &   MNIST   & EF-MNIST    & CIFAR10  &\vline &   MNIST   & EF-MNIST    & CIFAR10 \\    \hline
				
				NI-D  & 96 $\pm$0.3 & 78$\pm$1.1  & 79$\pm$0.5 &\vline & 96$\pm$0.3  & 78$\pm$1.1  & 79$\pm$0.5  &\vline& 96$\pm$0.3   & 78$\pm$1.1  & 79$\pm$0.5 \\
				
				NI & 97$\pm0.2$  & 82$\pm0.3$ & 80$\pm0.2$ &\vline & 97$\pm0.2$  & 82$\pm0.3$ & 80$\pm0.2$ &\vline& 97$\pm0.2$  & 82$\pm0.3$ & 80$\pm0.2$   \\
				\hline
				
				NISPA-Replay  & 77$\pm$1.2  & 66$\pm$1.4 & 38 $\pm$2.0   &\vline&  86$\pm$1.9  & 74$\pm$0.7 & 51$\pm$1.5  &\vline&  90$\pm$0.6 & 77$\pm$0.5  & 57$\pm$0.8 \\
				\hline
				
				DER  & 57$\pm$2.0  & 64$\pm$0.9 & 19$\pm$4.7   &\vline&  84$\pm$1.3  &77$\pm$0.3 & 30$\pm$9.9  &\vline&  87$\pm$0.9 & 79$\pm$0.6  & 33$\pm$1.2   \\
				
				ER  & 60$\pm$4.2  & 56$\pm$0.6 & 19$\pm$1.0   &\vline&  80$\pm$4.3  & 70$\pm$0.5 & 22$\pm$6.8  &\vline&  86$\pm$1.5 & 74$\pm$0.7  & 33$\pm$1.9  \\
				
				iCaRL & 73$\pm$1.4  & 51$\pm$0.6 & 40$\pm$2.7  &\vline&  74$\pm$1.9  & 45$\pm$0.7 & 47$\pm$2.5  &\vline&  61$\pm$3.7 & 57$\pm$0.2 & 30$\pm$1.8 \\
				
				A-Gem & 51$\pm$4.7  & 53$\pm$3.5 & 23$\pm$1.1   &\vline&  58$\pm$8.9  & 55$\pm$3.7 & 22$\pm$1.7  &\vline&  46$\pm$7.5 & 54$\pm$2.1  & 22$\pm$1.0  \\
				\hline
				
				DER-D & 73$\pm$4.0  & 71$\pm$0.4 & 25$\pm$1.0   &\vline&  90$\pm$1.2  & 80$\pm$0.4 & 31$\pm$10.7  &\vline&  93$\pm$2.0 & 81$\pm$0.4  & 39$\pm$14.5 \\
				
				ER-D & 69$\pm$1.2  & 60$\pm$0.6 & 22$\pm$0.7  &\vline&  87$\pm$0.8  & 73$\pm$0.4 & 22$\pm$9.9 &\vline&  90$\pm$0.6 & 76$\pm$0.3 & 41$\pm$1.3  \\
				
				iCaRL-D & 72$\pm$0.9  & 66$\pm$0.4 & 55$\pm$1.4   &\vline&  67$\pm$0.8  & 52$\pm$0.3 & 57$\pm$0.3  &\vline&  74$\pm$0.6 & 65$\pm$0.3  & 58$\pm$0.5  \\
			
				A-Gem-D & 40$\pm$6.3 & 55$\pm$1.8 & 22$\pm$1.5   &\vline&  26$\pm$2.9  & 56$\pm$1.6 & 28$\pm$0.7  &\vline&  32$\pm$9.4 & 51$\pm$4.4  & 23$\pm$0.6  \\
				
				\hline\noalign{\smallskip}	
				\hline\noalign{\smallskip}	    
	\end{tabular}}}
	\caption{Average accuracy across tasks after learning all tasks. Also, $\pm$ 1 std. is presented for average accuracies. Dense baselines are denoted with the suffix "-D" (e.g., DER-D or ER-D). Note that dense baselines have up to 10 times more learnable parameters, so they are significantly advantageous than NISPA. Therefore, they do not serve as a valid reference for benchmarking.}
	\label{tab:full}
\end{table*}
\endgroup

\subsection{Baselines}

\textbf{Experience Replay (ER): } This simple replay algorithm sequentially learns tasks while also training on small memory. It does not have any additional tricks. It uses the same loss function as NISPA. This method could be thought of as the lower bound for replay methods. Surprisingly, although its simplicity, this method has been shown to outperform complex CL approaches with memory replay \cite{DER, tiny-replay}. 

\textbf{Dark Experience Replay (DER): } This recent method is a simple extension to ER \cite{DER}. Similar to ER, it replays raw samples. The only difference is that instead of storing hard labels for the classes, it stores the logits of the trained model, and these logits are used as targets for replay samples. Although its simplicity, this method has been shown to outperform seven well-known replay-based methods by a large margin on several datasets \cite{DER}.

\textbf{iCaRL: } This is one of the most famous examples of replay methods \cite{icarl}. It relies on novel clustering-based classification, sample selection mechanism, and loss function.

\textbf{A-GEM: } This method is different than others as it stores raw samples but does not directly use them in training \cite{AGEM}. Instead, it projects gradients of novel tasks based on gradients computed for memory samples. However, like other baselines, it needs to store raw examples to compute gradients at a particular time in the training.
