# Supplementary material for: NISPA: Neuro-Inspired Stability-Plasticity Adaptation for Continual Learning in Sparse Networks
Source: arXiv:2206.09117 source file (2022-06-18)
Supplement: Supplementary file 6 [file 5_implementation_details.tex]

\section{Additional Details}

\subsection{NISPA in Convolutional Neural Networks:}
For the convolutional neural networks (CNNs), a unit stands for a 3D convolution filter. Likewise, each connection is represented by a 2D kernel instead of a single weight. Therefore, when we perform an operation, such as dropping or freezing a connection, we consider the entire 2D kernel representing the connection between two units. Note that this formulation reduces the FLOP count immensely by eliminating the operations performed on most 2D feature maps in units. Furthermore, units output a 2D matrix in a CNN instead of a scalar value. So, we consider the sum of all entries of this matrix as the activation of a unit. 

\subsection{Handling Corner Cases That Create Dead Units}
Our rewiring process rarely result in units without incoming (for stable units) or outgoing connections (for plastic units).
\begin{itemize}
    \item  If an plastic unit lost all of its outputs, we connect it to another plastic unit at the next layer. Unit at the next layer is chosen randomly.
    \item  Suppose an stable unit does not have incoming connections from stable units and, therefore, will lose all of its incoming connections during the rewiring. In that case, we degrade it to a plastic unit. 
\end{itemize}
The first correction step uses up the quota for random connection growing, so we still ensure that density stays exactly the same. 

\subsection{The Last Task}
We do not assume that we know the number of tasks beforehand. This leads to a subtle implementation detail. For example, if our algorithm knew which task was the final, it could select all free units as stable and use all the remaining capacity to perform well on the final task. However, since we do not assume such knowledge, our approach still selects the smallest number of stable units to have the capacity to learn further tasks. As a result, NISPA is always available for the next task in the CL setting.

\subsection{The Multi-Head Setting}
We have a multi-head setting. However, instead of replacing the head for each task, we have all of them initially. Interference is avoided by masking out activations (during training and testing) depending on the task. This is effectively the same with the multi-head setting, but having them all at once makes the growing algorithm straightforward for the penultimate layer. For example, when we drop incoming connections to Task 1 output units (stable units), in the growing part, we add connections from units at the penultimate layer to outputs of future tasks (plastic by definitions). In the last task, there are no plastic units at the output layer. So when we drop connections, we cannot add any connection back. So, density slightly decrease since we cannot grow some connections back.  However, the decrease in density is negligible. 
